# Supplementary material for: Learning long-range spatial dependencies with horizontal gated-recurrent units
Source: arXiv:1805.08315 source file (2019-06-11)
Supplement: Supplementary file 1 [file additional_treatment.tex]

\documentclass[12pt]{article}
\usepackage[margin=1in,bottom=1in,top=1in]{geometry}
\usepackage{polyglossia}
\usepackage{microtype}
\usepackage{fancyhdr}
\usepackage{amsmath}
\usepackage{mathtools}
\usepackage{amssymb}
\usepackage{tabu}
\usepackage{enumitem}
\usepackage{dsfont}
\usepackage{stmaryrd}
\usepackage[mathcal]{euscript}
\usepackage{scalerel,stackengine}
\usepackage{graphicx}
% \lhead{}
% \chead{}
% \rhead{}
\newcommand{\R}{\mathbb{R}}
\newcommand{\lp}{\left(}
\newcommand{\rp}{\right)}
\newcommand{\rb}{\right]}
\newcommand{\lb}{\left[}
% \fancyfoot{}
%%%%%%%%%%%%%%%%%%%%%%%%%%%%%%%%%%%%%%%%%%%%%%%%%%%%%%%%%%%%%%%%%%%%%%%%%%%%%
\begin{document}
\subsection*{Background on Euler's method}

Let $x(t):\R\to\R^n$ be an unknown function, and say that $\dot{x}:=\frac{dx}{dt}=f(x, t)$, where $f:\R^n\times\R\to\R^n$ is known. In other words, we have that
\[
\lim_{h\to0}\frac{x(t+h)-x(t)}{h}=f(x,t).
\]
Then, if $f$ is smooth enough and $h$ is very small,
\[
\frac{x(t+h)-x(t)}{h}\approx f(x,t).
\]
(Depending on $f$, this can be more true or less true, and you can prove different bounds on the error of approximation.) This is Euler's method: if we rearrange the equation, we get
\[
x(t+h)\approx x(t) + h f(x(t),t).
\]
So, we can come up with approximations $x[n]\approx x(nh)$ by iterating the step
\[
x[n]=x[n-1]+h f(x[n-1],t).
\]

\subsection*{Applied to Mély...}

Rewriting the simplified version of Mély's dynamical system in the form above, we obtain
\begin{align}
\dot{H}_{xyk}^{(1)} &= -\eta^{-1}\epsilon^2 H_{xyk}^{(1)} + \eta^{-1} \lb \xi X^k_{xy} - (\alpha H_{xyk}^{(1)} + \mu)C_{xyk}^{(1)}\rb_+\nonumber\\
\dot{H}_{xyk}^{(2)} &= -\eta^{-1}\sigma^2 H_{xyk}^{(2)} + \tau^{-1} \lb\gamma C_{xyk}^{(2)}\rb_+,
\end{align}
where $[\cdot]_+=\max(\cdot,0)$ is the ReLU function.

Now, we would like to simplify this equation, and then discretize it using Euler's method. First, choose $\eta=\tau$ and $\sigma=\epsilon$ since not all of these parameters are necessary for hGRU:
\begin{align*}
\dot{H}_{xyk}^{(1)} &= -\eta^{-1}\epsilon^2 H_{xyk}^{(1)} + \eta^{-1} \lb \xi X^k_{xy} - (\alpha H_{xyk}^{(1)} + \mu)C_{xyk}^{(1)}\rb_+\nonumber\\
\dot{H}_{xyk}^{(2)} &= -\eta^{-1}\epsilon^2 H_{xyk}^{(2)} + \eta^{-1} \lb \gamma C_{xyk}^{(2)}\rb_+,
\end{align*}
Now, apply Euler's method, with timestep $h$. This gives the iteration
\begin{align*}
H_{xyk}^{(1)}[n]&=H_{xyk}^{(1)}[n-1] + h \lp -\eta^{-1}\epsilon^2 H_{xyk}^{(1)}[n-1] + \eta^{-1} \lb \xi X^k_{xy}[n-1] - (\alpha H_{xyk}^{(1)}[n-1] + \mu)C_{xyk}^{(1)}[n-1]\rb_+\rp\\
H_{xyk}^{(2)}[n]&=H_{xyk}^{(2)}[n-1] + h \lp -\eta^{-1}\epsilon^2 H_{xyk}^{(2)}[n-1] + \eta^{-1}\lb\gamma C_{xyk}^{(2)}[n-1]\rb_+\rp.
\end{align*}
Distributing $h$,
\begin{align*}
H_{xyk}^{(1)}[n]&=H_{xyk}^{(1)}[n-1] - h \frac{\epsilon^2}{\eta} H_{xyk}^{(1)}[n-1] + h\eta^{-1} \lb \xi X^k_{xy}[n-1] - (\alpha H_{xyk}^{(1)}[n-1] + \mu)C_{xyk}^{(1)}[n-1]\rb_+\\
H_{xyk}^{(2)}[n]&=H_{xyk}^{(2)}[n-1] - h \frac{\epsilon^2}{\eta} H_{xyk}^{(2)}[n-1] + h \eta^{-1}\lb\gamma C_{xyk}^{(2)}[n-1]\rb_+.
\end{align*}
Now, notice that if we choose $h=\frac{\eta}{\epsilon^2}$, there first two terms on the RHS of each line will cancel:
\begin{align}
H_{xyk}^{(1)}[n]&=\epsilon^{-2}\lb \xi X^k_{xy}[n-1] - (\alpha H_{xyk}^{(1)}[n-1] + \mu)C_{xyk}^{(1)}[n-1]\rb_+\nonumber\\
H_{xyk}^{(2)}[n]&=\epsilon^{-2}\lb\gamma C_{xyk}^{(2)}[n-1]\rb_+.
\end{align}
This discrete-time dynamical system approximates Mély's system, but it can also be thought of as a fairly ordinary convolutional RNN with ReLU nonlinearity.
\end{document}
